# Supplementary material for: Spectral-Geometric Neural Fields for Pose-Free LiDAR View Synthesis
Source: arXiv:2603.12903 source file (2026-03-13)
Supplement: Supplementary file 1 [file X_suppl.tex]

\clearpage
\setcounter{page}{1}
\maketitlesupplementary

This supplement contains the following contents:

- More ablation studies and analysis.

- More experimental results.

- More implementation details.

\section{More Ablation Studies and Analysis}
\subsection{Efficacy of Cross-frame Consistency}
In Sec. 3.4, line 318 of the main paper, we introduce the Cross-frame Consistency (CFC) strategy, which leverages discriminative supervision to enhance reconstruction quality. Here, we provide additional experiments to demonstrate its efficacy. We evaluate our method with and without the CFC strategy on the low-frequency KITTI-360~\cite{liao2022kitti,xue2024geonlf} dataset in Table~\ref{tab:ablation_cfc} . Fig.~\ref{fig:cfc_visual} provides qualitative comparisons of the reconstructed depth maps in two consecutive frames.

SG-NLF ($w/o$ CFC) relies solely on pixel-level 2D depth image supervision ~\cite{zheng2024lidar4d,tao2024lidar}, as shown in Table ~\ref{tab:ablation_cfc}, resulting in a decrease in metrics. While 2D depth image supervision can oversee photometric alignment for each frame, it focuses more on pixel-wise improvements and ignores local structural information, leading to geometric breaks (\textit{e.g.}, incomplete telephone poles) and topological errors (\textit{e.g.}, incorrectly connected leaves), as shown by the rectanglar boxes in Fig.~\ref{fig:cfc_visual}. To overcome these issues, our CFC strategy introduces cross-frame structural discrimination. The discriminator is trained to identify geometric inconsistencies between aligned frames. When the model generates structurally inconsistent image pairs (\textit{e.g.}, poles not present in the predicted images but present in the ground truth cross-frame images), the discriminator classifies them as false. The resulting consistency loss $\mathcal{L}_{con}$ forces NeRF to reconstruct more consistent geometry in these regions, shown in the third row of Fig.~\ref{fig:cfc_visual}. These results demonstrate the effectiveness of our hybrid representation and cross-frame strategy in achieving robust reconstruction.

\subsection{Ablation on Sampling Points} 

We conduct ablation experiments on the number of sampling points ($M$) as described in Sec. 3.2 of main paper. As shown in Fig.~\ref{fig:supp_ablate_M}, we evaluate the reconstruction performance of depth RMSE and depth PSNR by varying $M$ from $512$ to $8192$. Reconstruction quality (depth RMSE and PSNR) is compromised with only $M=512$ points due to insufficient geometric coverage. Performance improves as $M$ grows and stabilizes beyond $4096$, indicating marginal gains from further increasing sampling density. Finally, we select the sampling points of $4096$, which can adequately meet the requirements of LiDAR scene reconstruction.
\begin{figure}[t]
    \centering
    \includegraphics[width=1\linewidth]{author-kit-CVPR2026-v1-latex-/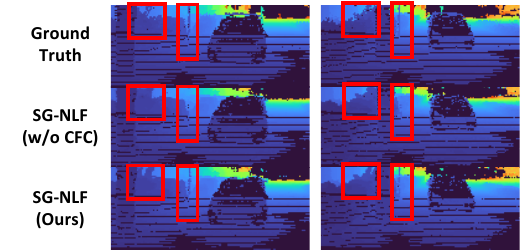}
    \caption{\textbf{Qualitative ablation of cross-frame consistency strategy.} We compare the reconstruction results of SG-NLF ($w/o$ CFC) and SG-NLF (Ours). SG-NLF ($w/o$ CFC) relies solely on pixel-level 2D depth image supervision. As shown in the rectangular boxes, while 2D depth image supervision ensures photometric alignment for each frame, it fails to preserve geometric details, resulting in incomplete telephone poles and incorrect leaf connections. By introducing cross-frame discrimination, our method learns cross-frame structure consistency representations, thus obtaining more complete and continuous reconstruction results.}
    \label{fig:cfc_visual}
\end{figure}

\begin{figure}[t]
    \centering
    \includegraphics[width=0.85\linewidth]{author-kit-CVPR2026-v1-latex-/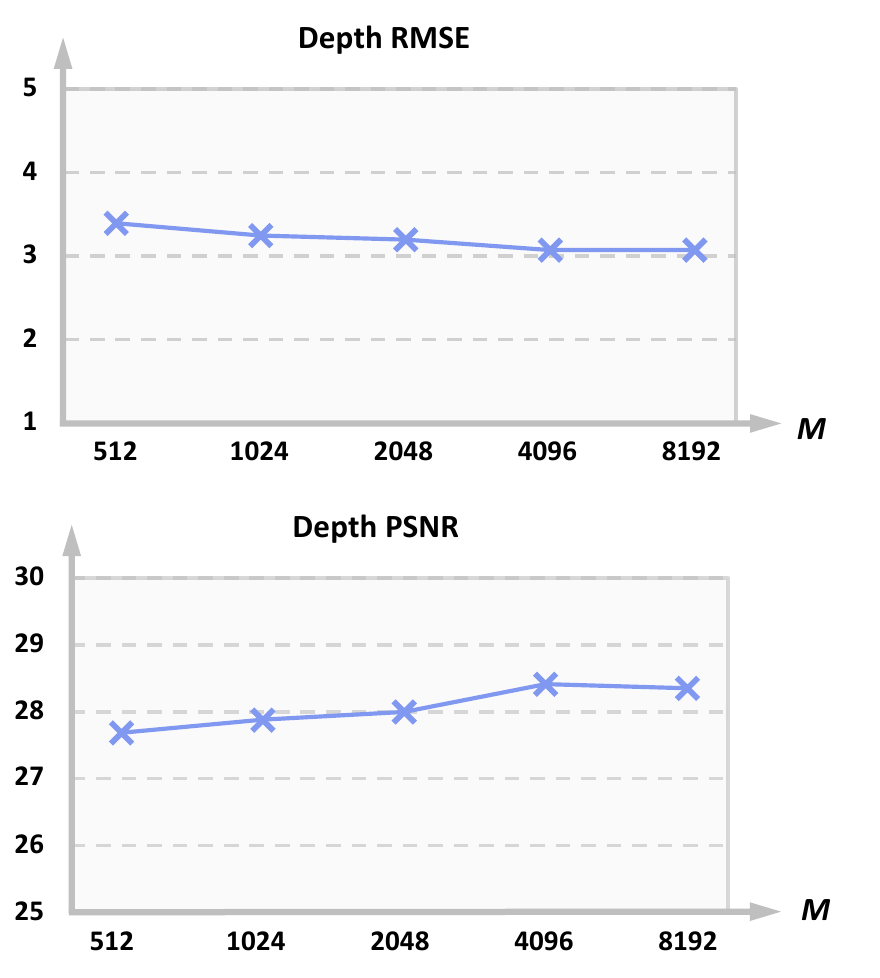}

    \caption{\textbf{Ablation experiments on the number of sampling points.} We evaluate the reconstruction performance of depth RMSE and depth PSNR by varying $M$ from $512$ to $8192$. Depth RMSE and PSNR are compromised with only $M=512$ points due to insufficient geometric coverage. Performance improves as $M$ grows and stabilizes beyond $4096$.}
    \label{fig:supp_ablate_M}
    \vspace{-10pt}
\end{figure}

\begin{table}[!t]
\caption{\textbf{Ablate on cross-frame consistency strategy (CFC).}  We evaluate our method with and without the CFC strategy on the low-frequency KITTI-360~\cite{liao2022kitti,xue2024geonlf} dataset. }
\begin{center}
\resizebox{\linewidth}{!}{
\begin{tabular}{lcccccc}
\toprule
 \multirow{2}*{Method} & \multirow{2}*{2D Range} & \multirow{2}*{CFC}& Point Cloud &  Depth& Intensity  \\
 & & &CD$\downarrow$   & PSNR$\uparrow$& PSNR$\uparrow$ \\
\midrule
SG-NLF($w/o$ CFC)& $\usym{2717}$&$\usym{2714}$ & 0.1735& 27.0587 & 18.2443  \\
SG-NLF(Ours) & $\usym{2714}$&$\usym{2714}$   & $\bold{0.1695}$& $\bold{28.7068}$ & $\bold{19.2652}$  \\
\bottomrule
\end{tabular}}
\end{center}
\label{tab:ablation_cfc}
\end{table}
\begin{figure*}[t]
    \centering
    \includegraphics[width=1\linewidth]{author-kit-CVPR2026-v1-latex-/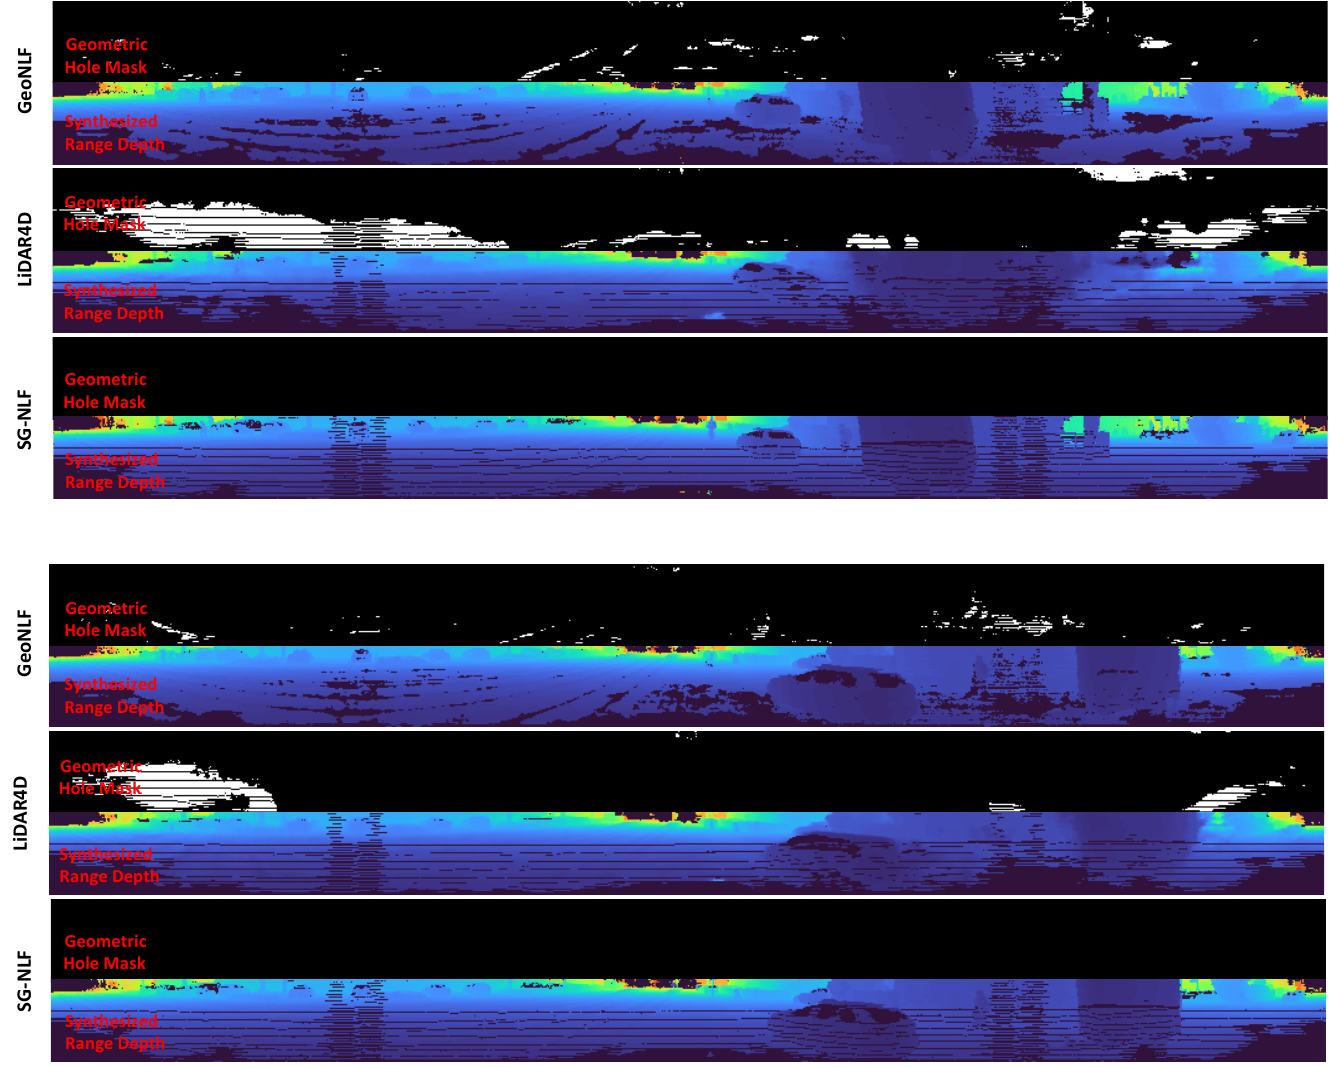}
    \caption{\textbf{Geometric Consistency Comparison.} The geometric hole mask is generated by comparing rendered opacity with ground truth LiDAR measurements. White regions  highlight geometric holes where methods fail to reconstruct geometry. GeoNLF~\cite{xue2024geonlf} and LiDAR4D~\cite{zheng2024lidar4d} exhibit significant geometric holes, resulting in blurred details and structural artifacts in the synthesized range depth maps. In contrast, our method achieves geometrically consistent reconstruction results with clear boundary, demonstrating our effectiveness.}
    \vspace{10pt}
    \label{fig:vis_hole}
\end{figure*}

\begin{table*}[t!]
\caption{\textbf{Comparisons on the standard-frequency KITTI-360~\cite{liao2022kitti} with challenging dynamic scenes~\cite{zheng2024lidar4d}.} We follow the setting of LiDAR4D~\cite{zheng2024lidar4d} and compare SG-NLF with state-of-the-art pose-dependent methods~\cite{manivasagam2020lidarsim,li2022pcgen,zheng2024lidar4d,huang2023nksr,tao2024lidar} and pose-free model~\cite{xue2024geonlf}. We color
the best results as \textcolor{red}{red} and the second-best as \textcolor{orange}{orange}.}

    \centering
    \resizebox{\textwidth}{!}{
    \begin{tabular}{lccccccccccccccc}

        \hline
        \multirow{2}*{Method}  & \multicolumn{3}{c}{Point Cloud} & \multicolumn{6}{c}{Depth} & \multicolumn{5}{c}{Intensity}\\
        \cmidrule{2-3} \cmidrule{5-9} \cmidrule{11-15}
                            & CD$\downarrow$ &F-score$\uparrow$& &RMSE$\downarrow$ & MedAE$\downarrow$ & LPIPS$\downarrow$& SSIM$\uparrow$& PSNR$\uparrow$ && RMSE$\downarrow$ & MedAE$\downarrow$ & LPIPS$\downarrow$& SSIM$\uparrow$& PSNR$\uparrow$\\
        \hline
        LiDARsim~\cite{manivasagam2020lidarsim}            & 3.2228 & 0.7157 & & 6.9153  & 0.1279  & 0.2926& 0.6342  & 21.4608 && 0.1666     & 0.0569   & 0.3276    & 0.3502  & 15.5853\\
        
        PCGen~\cite{li2022pcgen}         & 0.4636   & 0.8023 & & 5.6583  & 0.2040  & 0.5391  & 0.4903 & 23.1675 & & 0.1970     & 0.0763   & 0.5926   & 0.1351  & 14.1181\\
        NKSR~\cite{huang2023nksr} & 1.8982 & 0.6855 & &5.8403  & 0.0996   & 0.2752  & 0.6409 & 23.0368 & & 0.1742    & 0.0590   & 0.3337   & 0.3517 & 15.2081\\
        LiDAR-NeRF~\cite{tao2024lidar}            & 0.1438   &0.9091 & & 4.1753 & 0.0566 & 0.2797  & 0.6568 & 25.9878 & & 0.1404   & 0.0443     & 0.3135     & 0.3831   & 17.1549\\
        LiDAR4D~\cite{zheng2024lidar4d}           & \cellcolor{orange!40}0.1089     & \cellcolor{red!40}0.9272   & & 3.5256   & \cellcolor{red!40}0.0404    &\cellcolor{orange!40}0.1051   &0.7647    & 27.4767  && \cellcolor{orange!40}0.1195     & \cellcolor{orange!40}0.0327    & \cellcolor{red!40}0.1845   & \cellcolor{orange!40}0.5304    & \cellcolor{orange!40} 18.5561\\
        GeoNLF~\cite{xue2024geonlf}             & 0.2872   & 0.8766  && \cellcolor{orange!40}3.0218  & 0.0467  & 0.1343  & \cellcolor{orange!40}0.8002  & \cellcolor{orange!40}28.4861 && 0.1286     & 0.0402  & 0.2751  & 0.5025  &17.8174\\
        SG-NLF (Ours)            & \cellcolor{red!40}0.1047  & \cellcolor{orange!40} 0.9176 && \cellcolor{red!40}2.7705 & \cellcolor{orange!40}0.0492 & \cellcolor{red!40}0.1007 & \cellcolor{red!40}0.8351 &\cellcolor{red!40}29.6267& & \cellcolor{red!40}0.1069    &  \cellcolor{red!40} 0.0320   & \cellcolor{orange!40}0.2343  & \cellcolor{red!40}0.5894 & \cellcolor{red!40}19.4302\\
        \hline
    \end{tabular}}

    \label{tab:kitti_dynamic}

\end{table*}

\subsection{Comparison with Gaussian Splatting} 
SG-NLF also outperforms Gaussian-Splatting-based model GS-LiDAR~\cite{jiang2025gs} in the quality of LiDAR view synthesis. As discussed in the GS-LiDAR paper, current methods (\textit{e.g.}, LiDAR-NeRF, GeoNLF, LiDAR4D, etc.) adopt NeRF-based frameworks owing to their “effective implicit representation and high-quality volumetric rendering”. On the other hand, “3D Gaussian splatting struggles with geometric modeling and tends to overfit sparse views”. GS-LiDAR represents an initial effort to apply Gaussian primitives to this task. However, limited by the above challenges, as shown in the table below, our method surpasses GS-LiDAR by $11.2\%$ (Depth RMSE) and $7.9\%$ (Intensity RMSE) on KITTI-360 dataset. 

\begin{table}[t!]
\caption{\textbf{Comparisons on the standard-frequency KITTI-360~\cite{liao2022kitti}.}}

    \centering
    \resizebox{\linewidth}{!}{
\begin{tabular}{lcccccccccc}
\toprule
 \multirow{2}*{Method} & Point Cloud  & \multicolumn{4}{c}{Depth}&\multicolumn{2}{c}{Intensity} \\
 \cmidrule{2-2}  \cmidrule{4-5} \cmidrule{7-8} 
 & CD$\downarrow$  & & RMSE$\downarrow$  & PSNR$\uparrow$& &RMSE$\downarrow$ & PSNR$\uparrow$ \\
\midrule
GS-LiDAR (ICLR 2025)& 0.1085 &&3.1212	 &28.4381	&&0.1161 &18.7482 \\
SG-NLF (Ours)& \textbf{0.1047}&&\textbf{2.7705}& \textbf{29.6267}&& \textbf{0.1069} &\textbf{19.4302}
\\
\bottomrule
           
\end{tabular}}
%\caption{Reference frames numbers n.}
\end{table}

\section{More Experimental Results}
\subsection{Geometric Consistency Comparison}
As illustrated in Fig.~2 and line 061 of our submitted manuscript, previous approaches~\cite{xue2024geonlf,zheng2024lidar4d,tao2024lidar,huang2023neural} typically rely on geometric interpolation for neural field rendering.  However, due to the sparsity and irregularity of LiDAR data, such interpolated features often fail to reconstruct continuous surfaces, leading to geometric inconsistency. We provide further comparative visualization in Fig.~\ref{fig:vis_hole}.  We obtain the geometric hole mask by comparing the opacity of the model rendering with the actual LiDAR measurements. The white regions show areas where these methods fail to reconstruct the geometry. As shown in Fig.~\ref{fig:vis_hole}, geometric interpolation-based methods such as GeoNLF~\cite{xue2024geonlf} and LiDAR4D~\cite{zheng2024lidar4d} exhibit significant geometric holes, resulting in blurred details and structural artifacts in the synthesized range depth maps. In contrast, our method achieves geometrically consistent reconstruction results with clear boundaries, demonstrating the effectiveness of our SG-NLF.

\subsection{More Quantitative Results}
In Sec. 4.2 and Table 3 of the submitted main manuscript, we evaluate SG-NLF on the standard-frequency KITTI-360~\cite{liao2022kitti} dataset, demonstrating high-quality reconstruction and synthesis. Here, we extend our evaluation to challenging dynamic scenes, using the same settings as LiDAR4D~\cite{zheng2024lidar4d} on the standard-frequency KITTI-360 dataset~\cite{liao2022kitti}. LiDAR4D incorporates a scene flow prior to enhance reconstruction consistency in dynamic environments. As shown in Table~\ref{tab:kitti_dynamic}, even without employing the time prior for scene flow, SG-NLF improves depth SSIM, depth PSNR, intensity SSIM, and intensity PSNR by over 9.2\%, 7.8\%, 11.1\%, and 4.7\% than LiDAR4D~\cite{zheng2024lidar4d}, demonstrating the robustness and generalization of our framework.

\subsection{SG-NLF with Ground Truth Pose Input}
The advantages of our method compared to state-of-the-art pose-dependent methods~\cite{manivasagam2020lidarsim,li2022pcgen,zheng2024lidar4d} and pose-free models~\cite{xue2024geonlf,lin2021barf,heo2023robust} are demonstrated through Figures 4 to 6 and Tables 1 to 4 in our submitted manuscript. As analyzed in Sec. 4.2, our pose-independent SG-NLF achieves competitive performance without relying on the ground truth pose input, even outperforming pose-dependent models in challenging scenarios. To further demonstrate the efficacy of our hybrid representation, we conduct additional experiments with ground truth poses as input. Table~\ref{tab:ablation_kitti} and Table~\ref{tab:ablation_nus} provide comparative results on the low-frequency KITTI-360~\cite{liao2022kitti,xue2024geonlf} and low-frequency nuScenes~\cite{caesar2020nuScenes,xue2024geonlf} datasets. When ground truth poses are provided, our method achieves higher reconstruction accuracy, significantly surpassing the leading pose-dependent method LiDAR4D, demonstrating the effectiveness of our hybrid spectral-geometry design.

%------------------------------------------------------------------------
\begin{table*}
\caption{\textbf{More comparisons with state-of-the-art methods on KITTI-360~\cite{liao2022kitti} dataset with a low-frequency setting~\cite{xue2024geonlf}.} We conduct additional experiments with ground truth poses (GT Pose) as input. Compared to state-of-the-art pose-dependent methods~\cite{manivasagam2020lidarsim,li2022pcgen,zheng2024lidar4d,huang2023nksr}, our SG-NLF achieves better reconstruction performance when providing ground truth poses.}
    \centering
    \resizebox{\textwidth}{!}{
    \begin{tabular}{clccccccccccccccc}

        \hline
       Type &\multirow{2}*{Method}  & \multicolumn{3}{c}{Point Cloud} & \multicolumn{6}{c}{Depth} & \multicolumn{5}{c}{Intensity}\\
        \cmidrule{3-4} \cmidrule{6-10} \cmidrule{12-16}
                   GT Pose   &    & CD$\downarrow$ &F-score$\uparrow$& &RMSE$\downarrow$ & MedAE$\downarrow$ & LPIPS$\downarrow$& SSIM$\uparrow$& PSNR$\uparrow$ && RMSE$\downarrow$ & MedAE$\downarrow$ & LPIPS$\downarrow$& SSIM$\uparrow$& PSNR$\uparrow$\\
        \hline
       $\usym{2714}$ &LiDARsim~\cite{manivasagam2020lidarsim}                 & 11.0426  &0.5975 & & 10.1994  & 1.3881 & 0.5588 & 0.3888  & 17.9423 && 0.2089   &  0.1254  & 0.6463  & 0.0824  & 13.6127\\
       $\usym{2714}$ &PCGen~\cite{li2022pcgen}                 & 1.0356  &0.7862 & & 7.5672  & 0.7066 & 0.5333 & 0.3744  & 20.6219 && 0.2139    & 0.1063  & 0.5930 & 0.1070  & 13.4243\\
       $\usym{2714}$ &NKSR~\cite{huang2023nksr}  & 1.3989  &0.6753 & & 8.8172  & 1.5896 & 0.5821 & 0.4135  & 19.2937 && 0.2133    & 0.1381  & 0.6099 & 0.0707  & 13.4516\\
       $\usym{2714}$&LiDAR4D~\cite{zheng2024lidar4d}              & 0.2760  &0.8843 & & 4.7303  & 0.0785 & 0.3368 & 0.6197  & 24.7282 & &0.1459    & 0.0524  & 0.3883& 0.3406    & 16.9512\\ 
       $\usym{2717}$ &BARF-LN~\cite{lin2021barf,tao2024lidar}         & 3.1001  &0.6156 & & 7.5767  & 2.0583 & 0.5779 & 0.2834  & 22.5759& & 0.2121    & 0.1575  & 0.7121  & 0.1468  & 11.9778\\
       $\usym{2717}$ &HASH-LN~\cite{heo2023robust,tao2024lidar}   & 2.6913 & 0.6082 & & 6.3005 & 2.1686  & 0.5176 & 0.3752  & 22.6196& & 0.2404    & 0.1502   & 0.6508  & 0.1602 & 12.9286\\
       $\usym{2717}$ &GeoTrans-LN~\cite{qin2022geometric,tao2024lidar}           & 0.5753   & 0.8116 & & 4.4291  & 0.2023  & 0.3896  & 0.5330 & 25.6137  && 0.2709    & 0.1589   & 0.5578  & 0.2578  & 12.9707\\
        
       $\usym{2717}$ &GeoNLF~\cite{xue2024geonlf}                 & 0.2363   & 0.9178  && 4.0293  & 0.1009  & 0.3900  & 0.6272  & 25.2758 & & 0.1495     & 0.1525     & 0.5379    & 0.3165  & 16.5813\\
       \hline
 
      $\usym{2717}$ &SG-NLF(Ours)                  & \underline{0.1695}   & \underline{0.9191} && \underline{2.9514} & \underline{0.0544} &\underline{0.0701}  & \underline{0.9270}  & \underline{28.7068}  & &\underline{0.1089}     & \underline{0.0368}   &\underline{0.2026}  & \underline{0.5751}  &  \underline{19.2652}\\
       
      $\usym{2714}$ &SG-NLF(w/ pose)                  &$\bold{0.1180}$   & $\bold{0.9317}$ && $\bold{2.1510}$ &$\bold{0.0312}$ & $\bold{0.0424}$  &$ \bold{0.9532} $ & $\bold{31.4257} $ & &$\bold{0.1029}$     &$\bold{0.0363}$   & $\bold{0.1840}$  & $\bold{0.6185}$  & $\bold{19.7479}$\\
       \hline
    \end{tabular}}

    \label{tab:ablation_kitti}
\end{table*}

\subsection{More Qualitative Results}
We show more visual comparisons in Fig.~\ref{fig:vis_depthsupp}, ~\ref{fig:vis_intensupp}, and~\ref{fig:vis_pointsupp}. Fig.~\ref{fig:vis_depthsupp} provides qualitative comparisons for LiDAR depth reconstruction and synthesis, while Fig.~\ref{fig:vis_intensupp} presents comparisons for LiDAR intensity reconstruction and synthesis. We further visualize the reconstructed point clouds in Fig.~\ref{fig:vis_pointsupp}. 

\begin{figure*}[t]
    \centering
    \includegraphics[width=1\linewidth]{author-kit-CVPR2026-v1-latex-/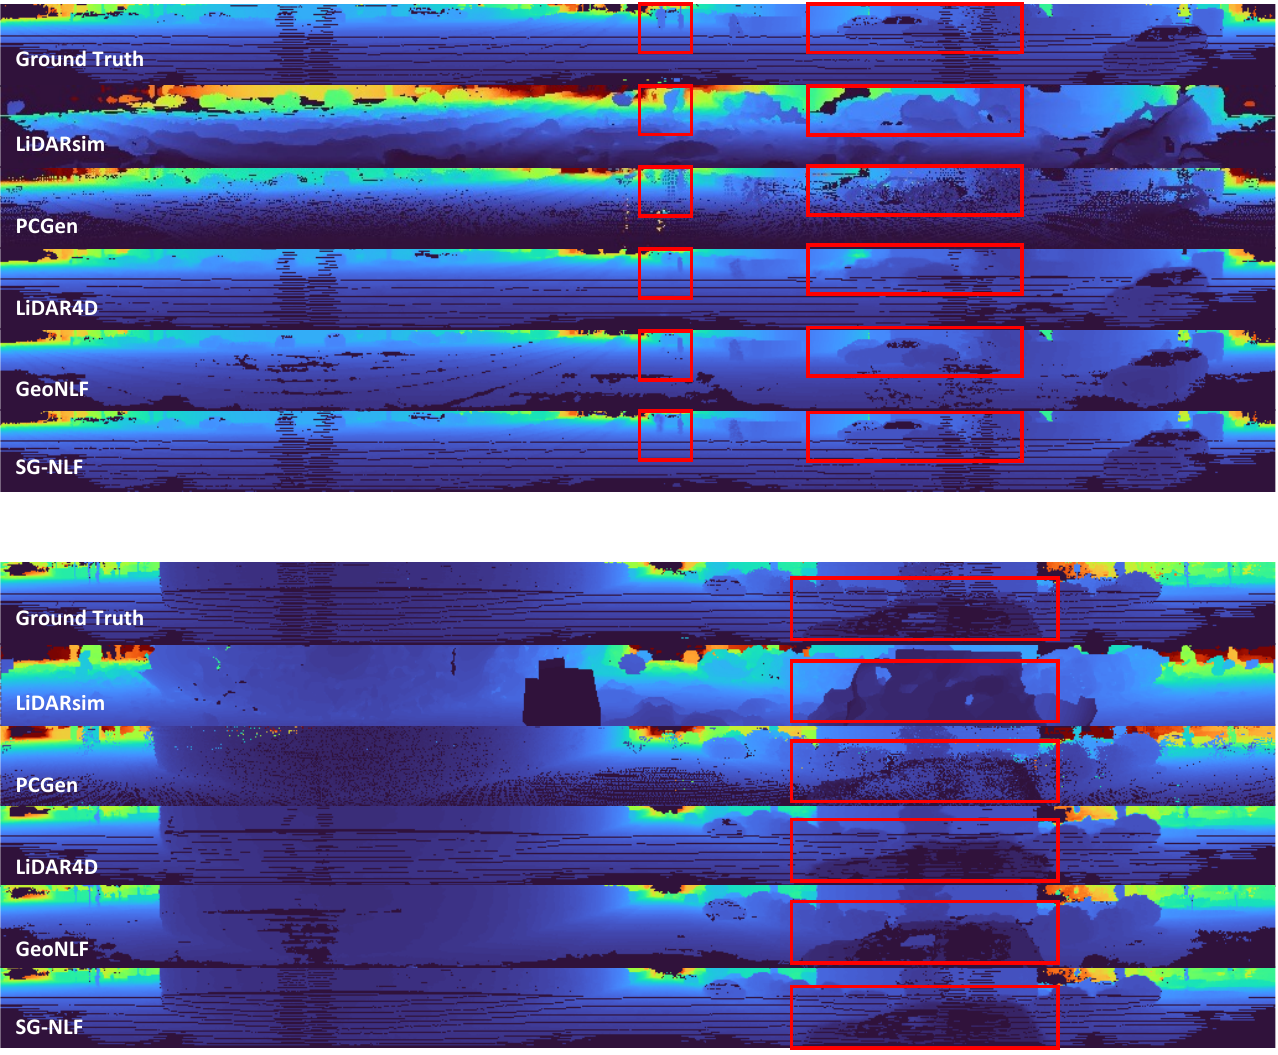}
    \caption{\textbf{Qualitative comparisons for LiDAR range depth reconstruction and synthesis.} Both pose-dependent~\cite{zheng2024lidar4d,li2022pcgen,huang2023nksr} and pose-free methods~\cite{xue2024geonlf} are compared. Regions with obvious differences are highlighted in the rectangular boxes.}
    \vspace{10pt}
    \label{fig:vis_depthsupp}
\end{figure*}

%----------------------------------------------------------
\begin{table*}
\caption{\textbf{More comparisons with state-of-the-art methods on nuScenes~\cite{caesar2020nuScenes} dataset with a low-frequency setting~\cite{xue2024geonlf}.} We conduct additional experiments with ground truth poses (GT Pose) as input. Compared to state-of-the-art pose-dependent methods~\cite{manivasagam2020lidarsim,li2022pcgen,zheng2024lidar4d,huang2023nksr}, our SG-NLF achieves better reconstruction performance when providing ground truth poses.}

    \centering
    \resizebox{\textwidth}{!}{
    \begin{tabular}{clccccccccccccccc}

        \hline
        Type &\multirow{2}*{Method}  & \multicolumn{3}{c}{Point Cloud} & \multicolumn{6}{c}{Depth} & \multicolumn{5}{c}{Intensity}\\
        \cmidrule{3-4} \cmidrule{6-10} \cmidrule{12-16}
                           GT Pose  &  &  CD$\downarrow$ &F-score$\uparrow$& &RMSE$\downarrow$ & MedAE$\downarrow$ & LPIPS$\downarrow$& SSIM$\uparrow$& PSNR$\uparrow$ && RMSE$\downarrow$ & MedAE$\downarrow$ & LPIPS$\downarrow$& SSIM$\uparrow$& PSNR$\uparrow$\\
        \hline
        $\usym{2714}$ &LiDARsim~\cite{manivasagam2020lidarsim}               & 16.7623  &0.4308 & & 12.3483  & 1.9971 & 0.3125 & 0.3889  & 16.2553 && 0.0858    & 0.0355  & 0.1713  & 0.2897  & 21.3989\\
        $\usym{2714}$ &PCGen~\cite{li2022pcgen}               & 2.2608  &0.6139  && 12.6586  &0.7055 &  0.2365 & 0.4389  & 12.6586& & 0.0865    & 0.0235  & 0.1530  & 0.3707  & 21.3643\\
        $\usym{2714}$ &NKSR~\cite{huang2023nksr}  & 2.4444  &0.5955 & &  13.2809  & 3.0977 & 0.3957 & 0.3373  & 15.6226 && 0.0910    & 0.0409  &  0.2079 & 0.2627  & 20.8796\\

        $\usym{2714}$ &LiDAR4D~\cite{zheng2024lidar4d}               & 0.5668  & 0.7444 & & 11.1964  & 0.0847 & 0.0685 & 0.5983  & 17.0920 && 0.0599    & 0.0180  & 0.0639 & 0.5401  & 24.4753\\   
        $\usym{2717}$ &BARF-LN~\cite{lin2021barf,tao2024lidar}               & 1.2695   & 0.7589 & & 8.2414   & 0.1123  & 0.1432  & 0.6856  & 20.8900 &  & 0.3920   & 0.0144    & 0.1023   & 0.6119 & 26.2330\\
        $\usym{2717}$ &HASH-LN~\cite{heo2023robust,tao2024lidar}             & 0.9691   & 0.8011 & & 7.8353  & 0.0441 & 0.1190  & 0.6543  & 20.6244 & & 0.0459     & 0.0135   & 0.0954  & 0.6279  & 26.8870\\
        $\usym{2717}$ &GeoTrans-LN~\cite{qin2022geometric,tao2024lidar}              & 4.1587    & 0.2993 &  & 10.7899   & 2.1529   & 0.1445   & 0.3671   & 17.5885 && 0.0679     & 0.0256  & 0.1149  & 0.3476  & 23.6211\\
         
        $\usym{2717}$ &GeoNLF~\cite{xue2024geonlf}              & 0.2408   & 0.8647   & &5.8208   & 0.0281   & 0.0727  & 0.7746   & 22.9472  & &0.0378      & 0.0100   & 0.0774   & 0.7368  & 28.6078\\
           \hline
 
        $\usym{2717}$ &SG-NLF(Ours)          & \underline{0.1545}  & \underline{0.9097} & &\underline{3.0706} &\underline{0.0278} &\underline{0.0191} &\underline{0.9398} &\underline{28.4094} &&\underline{0.0299}    & \underline{0.0078}   & \underline{0.0349}  & \underline{0.8679} & \underline{30.4987}\\
        $\usym{2714}$ &SG-NLF(w/ pose)          &$\bold{0.1078}$   & $\bold{0.9354}$ && $\bold{2.2764}$ &$\bold{0.0238}$ & $\bold{0.0107}$  &$ \bold{0.9467} $ & $\bold{31.2547} $ & &$\bold{0.0235}$     &$\bold{0.0056}$   & $\bold{0.0327}$  & $\bold{0.8964}$  & $\bold{31.0764}$\\
        \hline
    \end{tabular}}

    \label{tab:ablation_nus}
\end{table*}

\begin{figure*}[t]
    \centering
    \includegraphics[width=1\linewidth]{author-kit-CVPR2026-v1-latex-/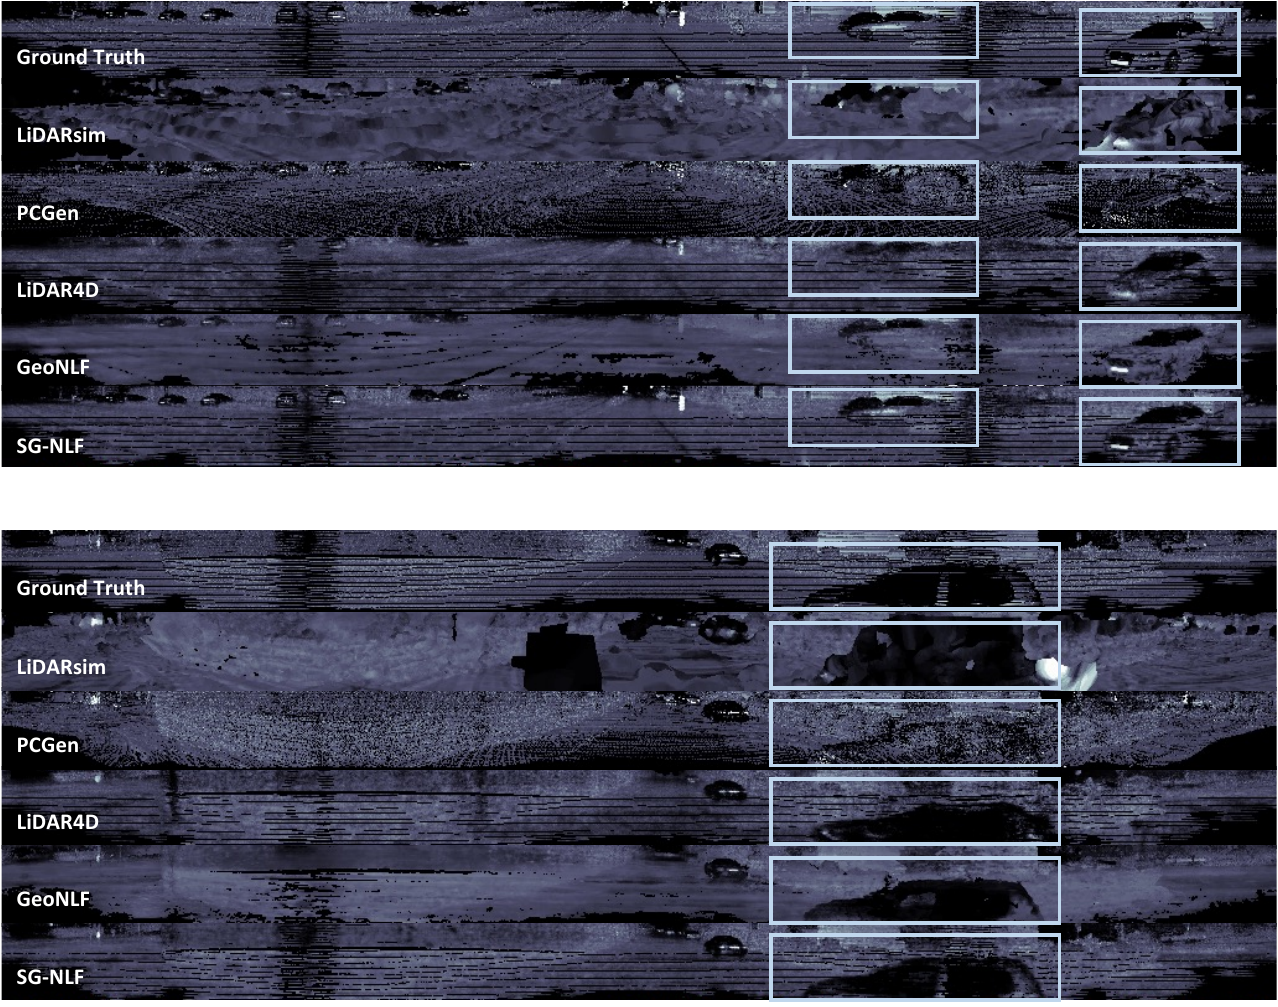}
    \caption{\textbf{Qualitative comparisons for LiDAR range intensity reconstruction and synthesis.} Both pose-dependent~\cite{zheng2024lidar4d,li2022pcgen,huang2023nksr} and pose-free methods~\cite{xue2024geonlf} are compared. Regions with obvious differences are highlighted in the rectangular boxes.}
    \label{fig:vis_intensupp}
\end{figure*}

\begin{figure*}[t]
    \centering
    \includegraphics[width=1\linewidth]{author-kit-CVPR2026-v1-latex-/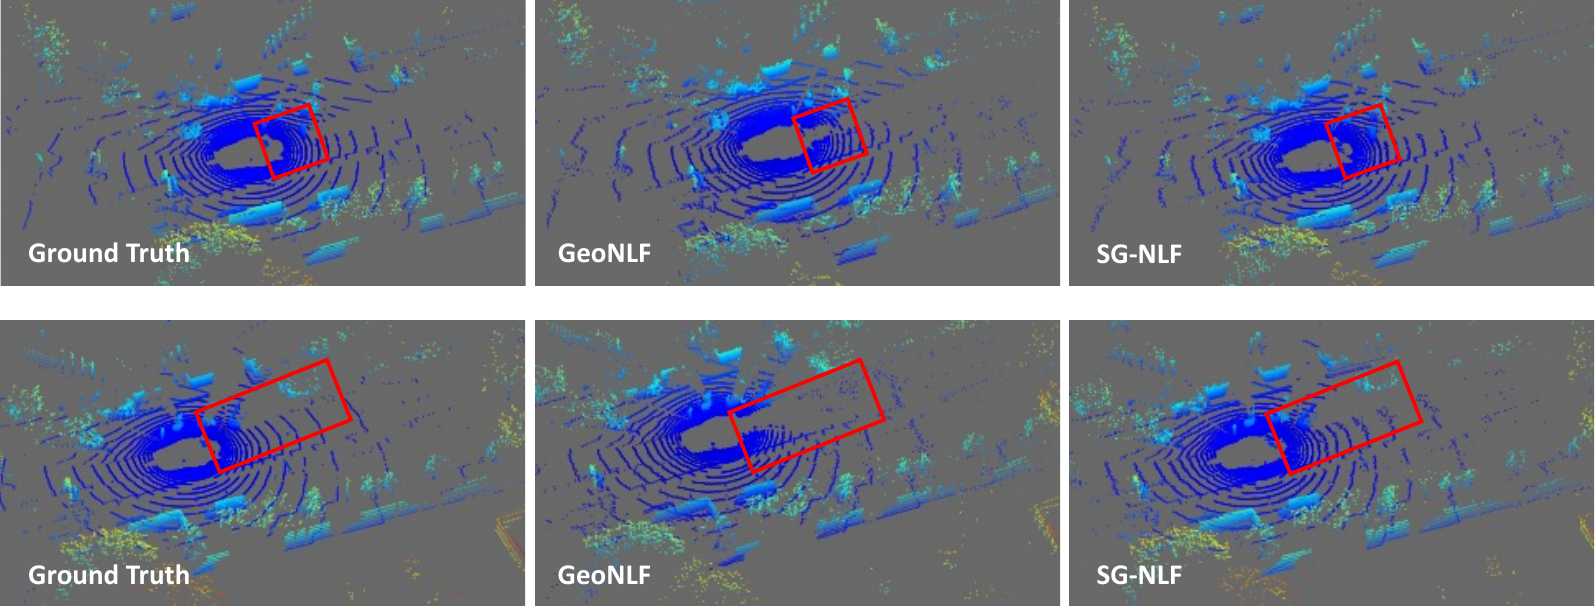}
    \caption{\textbf{Qualitative novel view LiDAR point cloud synthesis results on nuScenes~\cite{caesar2020nuScenes,xue2024geonlf} dataset.} The point clouds from each frame are visualized from a top-down (Bird's-Eye View) perspective for analysis. Comparative results demonstrate that our SG-NLF achieves more complete road reconstruction than GeoNLF~\cite{xue2024geonlf}, as highlighted by the red rectangular boxes.}
    \vspace{-5pt}
    \label{fig:vis_pointsupp}
\end{figure*}

\subsection{Model Efficiency}
In Fig. 1 of the submitted main manuscript, we present the average rendering time per sequence on low-frequency KITTI-360~\cite{liao2022kitti,xue2024geonlf} dataset. To further evaluate the model efficiency, we compare the model parameters of different methods~\cite{tao2024lidar,zheng2024lidar4d,xue2024geonlf} in Table~\ref{tab:ablation_model}. Our evaluation follows the standard protocol using official implementations of competing methods~\cite{tao2024lidar,zheng2024lidar4d,xue2024geonlf}. As shown in Table~\ref{tab:ablation_model}, LiDAR4D~\cite{zheng2024lidar4d} exhibits significant computational overhead with 53.1M parameters and 242$\,$ms runtime, primarily due to its complex planar-grid representation that introduces substantial memory. In contrast, our SG-NLF achieves a balance between performance and efficiency, with only 18.4M parameters (65\% reduction compared to LiDAR4D~\cite{zheng2024lidar4d}) and 20$\,$ms average inference time (over 12 times faster). 
\begin{table}[!t]
\caption{\textbf{Model efficiency. } We report model parameters (M) and runtime (ms) of different methods~\cite{tao2024lidar,zheng2024lidar4d,xue2024geonlf}. Our evaluation follows the standard protocol using official implementations of competing methods~\cite{tao2024lidar,zheng2024lidar4d,xue2024geonlf}.  Runtime are evaluated on the KITTI-360~\cite{liao2022kitti,xue2024geonlf} dataset, reporting the average rendering time per sequence. }
\vspace{-10pt}
\begin{center}
\resizebox{\linewidth}{!}{
\begin{tabular}{lcccc}
\toprule
&LiDAR4D~\cite{zheng2024lidar4d}& LiDAR-NeRF~\cite{tao2024lidar}& GeoNLF~\cite{xue2024geonlf} &   SG-NLF(Ours)\\
\midrule
Params (M)& 53.1& 13.6&18.3&18.4\\
Time (ms) &242&55&20&25\\
\bottomrule
\end{tabular}}
\vspace{-10pt}
\end{center}
\label{tab:ablation_model}
\end{table}

\subsection{Training time}Our SG-NLF is efficient without a
heavy training burden. We test on a 4090 GPU. (1) SG-NLF
takes 1.7 hours for training per scene, comparable to baselines like LiDAR4D (2.1 hours) and GeoNLF (1.6 hours).
(2) Original NeRF consumes 82\% of training time. Additional regularizations and networks only take up 18\%. 

\section{More Implementation Details}
Following Sec. 3.3, Sec. 3.4, and Sec. 4.1 of the submitted main manuscript, we present more detailed descriptions of our framework and implementations.

\subsection{Hybrid Spectral-Geometric Representation}
For geometric encoding, we use a hash grid with $20$ levels, each level displaying $2$-dimensional features, resulting in the same $40$-dimensional features. The grid is mapped to a $2^{19}$ hash table. For spectral embedding, we use a 3-layer MLP for spherical mapping and another 3-layer MLP to learn the $K=8$ eigenfunctions. We perform area-weighted sampling and select $M=4096$ points for the spectral loss computation. Geometric encoding and spectral embedding constitute a $48$-dimensional latent vector.

The fused spectral-geometric features are fed into a $2$-layer $64$-dimensional MLP, producing a $20$-dimensional intrinsic feature vector and density value. The intrinsic features, combined with 12-band frequency-coded viewpoint information, are then fed into two independent $3$-layer $64$-dimensional MLPs to predict intensity values and ray-drop probabilities, respectively. The expectation of the density integrated along the ray serves as the depth value.

\subsection{Global Pose Optimization}
Beyond hybrid spectral-geometric representation for scene reconstruction, we additionally design a dynamically constructed graph for pose optimization. The edge inclusion threshold $\theta$ increases linearly from $0.5$ to $0.9$ during training to enforce progressively stricter edge selection. Similarly, the distance preservation threshold $\tau_d$ increases from $0.1$ to $0.2$ to accommodate improving alignment quality. For each edge $(i,j) \in \mathcal{E}$ in the pose graph, we compute the Chamfer Distance between the transformed point clouds:
\begin{equation}
\small
\mathcal{L}_{\text{cd}}^{ij} = \frac{1}{|\mathcal{S}_i|} \sum_{\mathbf{x} \in \mathcal{S}_i} \min_{\mathbf{y} \in \mathcal{S}_j} \|\mathbf{x} - \mathbf{y}\|_2^2 + \frac{1}{|\mathcal{S}_j|} \sum_{\mathbf{y} \in \mathcal{S}_j} \min_{\mathbf{x} \in \mathcal{S}_i} \|\mathbf{x} - \mathbf{y}\|_2^2\,,
\end{equation}
where $\mathcal{S}_i$ and $\mathcal{S}_j $ represent the point clouds transformed by the optimized poses. The final pose graph loss combines the weighted Chamfer Distance across all edges:
\begin{equation}
\mathcal{L}_\text{graph} = \sum_{(i,j)\in \mathcal{E}} \alpha^{ij} \cdot \mathcal{L}_{\text{cd}}^{ij}\,.
\end{equation}

\subsection{Cross-frame Consistency}
For cross-frame consistency supervision, the projected range images are fed into a $4$-layer convolutional discriminator that outputs a 2D patch-wise authenticity map. The discriminator uses $64$ base channels with a kernel size of $4$ and stride of $2$, doubling the number of channels in each layer. The discriminator is trained to distinguish between geometrically consistent reconstructions and inconsistent ones by analyzing local patches at multiple scales, enabling it to capture both fine-grained details and global structural coherence. Furthermore, we supervise the neural LiDAR fields using the 2D range image loss~\cite{zheng2024lidar4d}:
\begin{equation}
\begin{aligned} \mathcal{L}_{ran}(\mathbf{r}) = &\sum_{\mathbf{r} \in R} \lambda_d\|\hat{D}(\mathbf{r}) - D(\mathbf{r})\|_1 + \sum_{\mathbf{r} \in R} \lambda_i\|\hat{I}(\mathbf{r}) - I(\mathbf{r})\|_2^2 \\
+ &\sum_{\mathbf{r} \in R} \lambda_p\|\hat{P}(\mathbf{r}) - P(\mathbf{r})\|_2^2\,,   
\end{aligned}
\end{equation}
where $\hat{D}$, $\hat{I}$, and $\hat{P}$ represent the predicted depth, intensity, and ray-drop probability respectively, while $D$, $I$, and $P$ denote the corresponding ground truth values. 

\subsection{Optimization Details}
Following prior pose-free methods~\cite{xue2024geonlf}, we adopt an alternating optimization strategy to achieve stable convergence. The process alternates between optimizing the neural LiDAR field parameters (for reconstruction) and refining the frame poses (for registration). After every $m_1$ epochs of neural LiDAR fields optimization, we perform $m_2$ epochs of pose optimization, with the ratio $m_2/m_1$ decreasing from 10 to 1 during training~\cite{xue2024geonlf}. The learning rate for pose optimization is synchronized with the neural field optimizer, following the same schedule as GeoNLF~\cite{xue2024geonlf}. The training objective for neural LiDAR fields combines consistency loss, range image loss, and spectral loss with the following weights: $\lambda_d = 20$ for depth, $\lambda_i = 0.5$ for intensity, $\lambda_n = 0.1$ and $\lambda_o = 10$ for spectral components, and $1$ for other terms. The overall spectral loss weight increases progressively from 0 to 1 during training. Other unmentioned optimization details are basically in line with GeoNLF~\cite{xue2024geonlf}.
